# Supplementary material for: Static Electric Dipole Polarizability and Hyperpolarizability Tensors from Mean-Field Cavity Quantum Electrodynamics Approaches
Source: arXiv:2506.00217 ancillary file (2025-07-30)
Supplement: Supplementary file 1 [file si.pdf]

# Supporting Information for Static Electric Dipole Polarizability and Hyperpolarizability Tensors from Mean-Field Cavity Quantum Electrodynamics Approaches

A. Eugene DePrince III[a] and Stephen H. Yuwono

*Department of Chemistry and Biochemistry, Florida State University, Tallahassee, FL 32306-4390, USA*

[a]Electronic mail: adeprince@fsu.edu

## S1. CARTESIAN COORDINATES OF *P*-NITROANILINE IN Å

HF/d-aug-cc-pVTZ

| | X | Y | Z |
|---|---|---|---|
| C | 1.203224934805 | 0.000000000000 | -1.423902554313 |
| C | 1.201264001011 | 0.000000000000 | -0.052173381082 |
| C | 0.000000000000 | 0.000000000000 | 0.631184723059 |
| C | -1.201264001011 | 0.000000000000 | -0.052173381082 |
| C | -1.203224934805 | 0.000000000000 | -1.423902554313 |
| C | 0.000000000000 | 0.000000000000 | -2.134657980243 |
| N | 0.000000000000 | 0.000000000000 | -3.493778329651 |
| N | 0.000000000000 | 0.000000000000 | 2.079210059804 |
| O | 1.050837202880 | 0.000000000000 | 2.634967041381 |
| O | -1.050837202880 | 0.000000000000 | 2.634967041381 |
| H | 2.135384916544 | 0.000000000000 | -1.955199698726 |
| H | 2.121675479119 | 0.000000000000 | 0.492421181647 |
| H | -2.121675479119 | 0.000000000000 | 0.492421181647 |
| H | -2.135384916544 | 0.000000000000 | -1.955199698726 |
| H | -0.846585294537 | 0.000000000000 | -4.002624528884 |
| H | 0.846585294537 | 0.000000000000 | -4.002624528884 |

SVWN/d-aug-cc-pVTZ

| | X | Y | Z |
|---|---|---|---|
| C | 1.205921499901 | 0.000000000000 | -1.422241984865 |
| C | 1.205226468193 | 0.000000000000 | -0.050822369185 |
| C | 0.000000000000 | 0.000000000000 | 0.629965707862 |
| C | -1.205226468193 | 0.000000000000 | -0.050822369185 |
| C | -1.205921499901 | 0.000000000000 | -1.422241984865 |
| C | 0.000000000000 | 0.000000000000 | -2.134839653549 |
| N | 0.000000000000 | 0.000000000000 | -3.485720474889 |
| N | 0.000000000000 | 0.000000000000 | 2.064604247809 |
| O | 1.083340942335 | 0.000000000000 | 2.634805929420 |

```
O -1.083340942335  0.000000000000  2.634805929420
H  2.151371956864  0.000000000000 -1.970439242123
H  2.128187270969  0.000000000000  0.531149847027
H -2.128187270969  0.000000000000  0.531149847027
H -2.151371956864  0.000000000000 -1.970439242123
H -0.868518349628  0.000000000000 -4.005586385573
H  0.868518349628  0.000000000000 -4.005586385573
```

PBE/d-aug-cc-pVTZ

```
   X                Y                Z
C  1.216078657857  0.000000000000 -1.441943299135
C  1.215429230926  0.000000000000 -0.056935072671
C  0.000000000000  0.000000000000  0.634983558177
C -1.215429230926  0.000000000000 -0.056935072671
C -1.216078657857  0.000000000000 -1.441943299135
C  0.000000000000  0.000000000000 -2.163340314318
N  0.000000000000  0.000000000000 -3.531432588296
N  0.000000000000  0.000000000000  2.095548289992
O  1.095783918353  0.000000000000  2.674695714898
O -1.095783918353  0.000000000000  2.674695714898
H  2.163254626339  0.000000000000 -1.984050713022
H  2.145480188182  0.000000000000  0.508356964897
H -2.145480188182  0.000000000000  0.508356964897
H -2.163254626339  0.000000000000 -1.984050713022
H -0.865016716372  0.000000000000 -4.052499510575
H  0.865016716372  0.000000000000 -4.052499510575
```

B3LYP/d-aug-cc-pVTZ

```
   X                Y                Z
C  1.209898375323  0.000000000000 -1.435562317242
C  1.209606253741  0.000000000000 -0.056525302675
C  0.000000000000  0.000000000000  0.632041628061
```

| | | | |
|---|---|---|---|
| C | -1.209606253741 | 0.000000000000 | -0.056525302675 |
| C | -1.209898375323 | 0.000000000000 | -1.435562317242 |
| C | 0.000000000000 | 0.000000000000 | -2.153320803602 |
| N | 0.000000000000 | 0.000000000000 | -3.518978853734 |
| N | 0.000000000000 | 0.000000000000 | 2.088053775422 |
| O | 1.083623174490 | 0.000000000000 | 2.663623112263 |
| O | -1.083623174490 | 0.000000000000 | 2.663623112263 |
| H | 2.149353190288 | 0.000000000000 | -1.972537171552 |
| H | 2.134146484769 | 0.000000000000 | 0.499372482213 |
| H | -2.134146484769 | 0.000000000000 | 0.499372482213 |
| H | -2.149353190288 | 0.000000000000 | -1.972537171552 |
| H | -0.857881557896 | 0.000000000000 | -4.036742989408 |
| H | 0.857881557896 | 0.000000000000 | -4.036742989408 |

$\omega$B97X/d-aug-cc-pVTZ

| | X | Y | Z |
|---|---|---|---|
| C | 1.206672419391 | 0.000000000000 | -1.432161796429 |
| C | 1.206385999502 | 0.000000000000 | -0.054868654327 |
| C | 0.000000000000 | -0.000000000000 | 0.626779100855 |
| C | -1.206385999502 | -0.000000000000 | -0.054868654327 |
| C | -1.206672419391 | -0.000000000000 | -1.432161796429 |
| C | 0.000000000000 | -0.000000000000 | -2.145174263304 |
| N | 0.000000000000 | -0.000000000000 | -3.510366596404 |
| N | 0.000000000000 | -0.000000000000 | 2.086849108319 |
| O | 1.073373057474 | 0.000000000000 | 2.654386858777 |
| O | -1.073373057474 | -0.000000000000 | 2.654386858777 |
| H | 2.145697147364 | 0.000000000000 | -1.971604074566 |
| H | 2.130695855749 | 0.000000000000 | 0.504274796348 |
| H | -2.130695855749 | -0.000000000000 | 0.504274796348 |
| H | -2.145697147364 | -0.000000000000 | -1.971604074566 |
| H | -0.857931715495 | -0.000000000000 | -4.024838753475 |
| H | 0.857931715495 | 0.000000000000 | -4.024838753475 |

TABLE S1. Mean-field energies at different coupling strengths ($\lambda$, in a.u.) and cavity polarization directions, using a cavity frequency of 0.1 $E_h$ ($\approx$ 2.72 eV).

| Cavity polarization | $\lambda$ | UHF | SVWN | PBE | B3LYP | $\omega$B97X |
|---|---|---|---|---|---|---|
| None | 0 | −489.394954 | −489.708816 | −491.752569 | −492.305459 | −492.166396 |
| | 0.01 | −489.392916 | −489.706595 | −491.750322 | −492.303276 | −492.164257 |
| | 0.02 | −489.386809 | −489.699944 | −491.743595 | −492.296736 | −492.157850 |
| $x$ | 0.03 | −489.376657 | −489.688897 | −491.732423 | −492.285872 | −492.147201 |
| | 0.04 | −489.362496 | −489.673507 | −491.716862 | −492.270732 | −492.132351 |
| | 0.05 | −489.344375 | −489.653847 | −491.696988 | −492.251384 | −492.113357 |
| | 0.01 | −489.393401 | −489.707286 | −491.751033 | −492.303922 | −492.164870 |
| | 0.02 | −489.388748 | −489.702701 | −491.746431 | −492.299316 | −492.160294 |
| $y$ | 0.03 | −489.381006 | −489.695073 | −491.738775 | −492.291654 | −492.152682 |
| | 0.04 | −489.370196 | −489.684421 | −491.728086 | −492.280955 | −492.142051 |
| | 0.05 | −489.356343 | −489.670774 | −491.714394 | −492.267249 | −492.128430 |
| | 0.01 | −489.392897 | −489.706399 | −491.750138 | −492.303154 | −492.164227 |
| | 0.02 | −489.386744 | −489.699208 | −491.742907 | −492.296281 | −492.157742 |
| $z$ | 0.03 | −489.376539 | −489.687400 | −491.731039 | −492.284958 | −492.147007 |
| | 0.04 | −489.362350 | −489.671185 | −491.714750 | −492.269345 | −492.132118 |
| | 0.05 | −489.344261 | −489.650778 | −491.694256 | −492.249612 | −492.113187 |

TABLE S2. Isotropically averaged static polarizabilities ($\bar{\alpha}$, in a.u.) and hyperpolarizabilities ($\bar{\beta}$, in a.u.) at different coupling strengths ($\lambda$, in a.u.) and cavity polarization directions, using a cavity frequency of 0.1 $E_h$ ($\approx$ 2.72 eV).

| Cavity polarization | $\lambda$ | $\bar{\alpha}$ | | | | | $\bar{\beta}$ |
|---|---|---|---|---|---|---|---|
| | | UHF | SVWN | PBE | B3LYP | $\omega$B97X | UHF |
| None | 0 | 93.795 | 109.802 | 112.245 | 106.641 | 100.994 | −133.465 |
| | 0.01 | 93.777 | 109.769 | 112.210 | 106.618 | 100.979 | −133.870 |
| | 0.02 | 93.725 | 109.675 | 112.109 | 106.552 | 100.937 | −135.067 |
| $x$ | 0.03 | 93.645 | 109.531 | 111.955 | 106.451 | 100.874 | −137.004 |
| | 0.04 | 93.541 | 109.350 | 111.764 | 106.329 | 100.798 | −139.600 |
| | 0.05 | 93.424 | 109.145 | 111.552 | 106.197 | 100.719 | −142.764 |
| | 0.01 | 93.760 | 109.758 | 112.196 | 106.598 | 100.956 | −133.620 |
| | 0.02 | 93.656 | 109.630 | 112.053 | 106.469 | 100.843 | −134.073 |
| $y$ | 0.03 | 93.487 | 109.422 | 111.822 | 106.262 | 100.659 | −134.780 |
| | 0.04 | 93.261 | 109.144 | 111.516 | 105.986 | 100.413 | −135.687 |
| | 0.05 | 92.985 | 108.807 | 111.146 | 105.651 | 100.111 | −136.733 |
| | 0.01 | 93.706 | 109.528 | 111.938 | 106.397 | 100.849 | −132.039 |
| | 0.02 | 93.446 | 108.737 | 111.058 | 105.699 | 100.431 | −127.917 |
| $z$ | 0.03 | 93.040 | 107.520 | 109.722 | 104.645 | 99.789 | −121.525 |
| | 0.04 | 92.521 | 106.020 | 108.102 | 103.364 | 98.989 | −113.477 |
| | 0.05 | 91.920 | 104.388 | 106.371 | 101.977 | 98.078 | −104.433 |

TABLE S3. Excitation energies and oscillator strengths characterizing the bright $A_1$ state of $p$-nitroaniline obtained with different levels of theory.

| Method | Excitation energy | | Oscillator strength |
|---|---|---|---|
| | $E_h$ | eV | |
| UHF | 0.192085 | 5.23 | 0.325958 |
| SVWN | 0.130665 | 3.56 | 0.282761 |
| PBE | 0.127421 | 3.47 | 0.271795 |
| B3LYP | 0.143849 | 3.91 | 0.335333 |
| $\omega$B97X | 0.170923 | 4.65 | 0.398725 |

TABLE S4. Mean-field energies at different cavity frequencies ($\omega_{\rm cav}$, in eV), using a coupling strength of 0.05 a.u. and cavity polarization along the $z$ axis.

| $\omega_{\rm cav}$ | UHF | SVWN | PBE | B3LYP | $\omega$B97X |
|---|---|---|---|---|---|
| 2.0 | −489.344261 | −489.650778 | −491.694256 | −492.249612 | −492.113817 |
| 3.0 | −489.344261 | −489.650778 | −491.694256 | −492.249612 | −492.113817 |
| 4.0 | −489.344261 | −489.650778 | −491.694256 | −492.249612 | −492.113817 |
| 5.0 | −489.344261 | −489.650778 | −491.694256 | −492.249612 | −492.113817 |
| 6.0 | −489.344261 | −489.650778 | −491.694256 | −492.249612 | −492.113817 |
| $\omega_{\rm res}$ [a] | −489.344261 | −489.650778 | −491.694256 | −492.249612 | −492.113817 |

[a] Cavity frequency that is resonant to the bright $A_1$ states as listed in Table S3.

TABLE S5. Isotropically averaged static polarizabilities ($\bar{\alpha}$, in a.u.) and hyperpolarizabilities ($\bar{\beta}$, in a.u.) at different cavity frequencies ($\omega_{\text{cav}}$, in eV), using a coupling strength of 0.05 a.u. and cavity polarization along the $z$ axis.

| $\omega_{\text{cav}}$ | $\bar{\alpha}$ | | | | | $\bar{\beta}$ |
|---|---|---|---|---|---|---|
| | UHF | SVWN | PBE | B3LYP | $\omega$B97X | UHF |
| 2.0 | 91.920 | 104.388 | 106.371 | 101.977 | 98.078 | −104.433 |
| 3.0 | 91.920 | 104.388 | 106.371 | 101.977 | 98.078 | −104.433 |
| 4.0 | 91.920 | 104.388 | 106.371 | 101.977 | 98.078 | −104.433 |
| 5.0 | 91.920 | 104.388 | 106.371 | 101.977 | 98.078 | −104.433 |
| 6.0 | 91.920 | 104.388 | 106.371 | 101.977 | 98.078 | −104.433 |
| $\omega_{\text{res}}$ [a] | 91.920 | 104.388 | 106.371 | 101.977 | 98.078 | −104.433 |

[a] Cavity frequency that is resonant to the bright $A_1$ states as listed in Table S3.

TABLE S6. Isotropically averaged static polarizabilities ($\bar{\alpha}$, in a.u.) at different coupling strengths ($\lambda$, in a.u.), cavity polarization directions, and basis sets, using a cavity frequency of 0.1 $E_h$ ($\approx$ 2.72 eV).

| Cavity polarization | $\lambda$ | cc-pV$n$Z | | | aug-cc-pV$n$Z | | | d-aug-cc-pV$n$Z | | |
|---|---|---|---|---|---|---|---|---|---|---|
| | | $n=$ D | $n=$ T | $n=$ Q | $n=$ D | $n=$ T | $n=$ Q | $n=$ D | $n=$ T | $n=$ Q |
| None | 0 | 77.788 | 85.668 | 89.896 | 93.423 | 93.723 | 93.755 | 93.886 | 93.795 | 93.775 |
| | 0.01 | 77.788 | 85.666 | 89.890 | 93.406 | 93.705 | 93.737 | 93.868 | 93.777 | 93.757 |
| | 0.02 | 77.789 | 85.658 | 89.873 | 93.357 | 93.653 | 93.685 | 93.815 | 93.725 | 93.705 |
| $x$ | 0.03 | 77.792 | 85.647 | 89.846 | 93.281 | 93.571 | 93.603 | 93.732 | 93.645 | 93.625 |
| | 0.04 | 77.798 | 85.635 | 89.812 | 93.183 | 93.466 | 93.499 | 93.627 | 93.541 | 93.522 |
| | 0.05 | 77.808 | 85.622 | 89.774 | 93.069 | 93.345 | 93.380 | 93.509 | 93.424 | 93.405 |
| | 0.01 | 77.783 | 85.659 | 89.880 | 93.389 | 93.688 | 93.720 | 93.850 | 93.760 | 93.739 |
| | 0.02 | 77.770 | 85.631 | 89.831 | 93.289 | 93.585 | 93.616 | 93.745 | 93.656 | 93.635 |
| $y$ | 0.03 | 77.747 | 85.584 | 89.751 | 93.127 | 93.418 | 93.449 | 93.575 | 93.487 | 93.467 |
| | 0.04 | 77.715 | 85.520 | 89.639 | 92.911 | 93.194 | 93.223 | 93.348 | 93.261 | 93.242 |
| | 0.05 | 77.675 | 85.437 | 89.498 | 92.646 | 92.921 | 92.949 | 93.073 | 92.985 | 92.966 |
| | 0.01 | 77.723 | 85.601 | 89.825 | 93.336 | 93.636 | 93.667 | 93.794 | 93.706 | 93.685 |
| | 0.02 | 77.535 | 85.406 | 89.617 | 93.085 | 93.381 | 93.410 | 93.528 | 93.446 | 93.426 |
| $z$ | 0.03 | 77.239 | 85.099 | 89.289 | 92.690 | 92.981 | 93.007 | 93.112 | 93.040 | 93.022 |
| | 0.04 | 76.856 | 84.701 | 88.864 | 92.181 | 92.466 | 92.491 | 92.581 | 92.521 | 92.504 |
| | 0.05 | 76.395 | 84.237 | 88.369 | 91.588 | 91.869 | 91.892 | 91.968 | 91.920 | 91.905 |

TABLE S7. Isotropically averaged static hyperpolarizabilities ($\bar{\beta}$, in a.u.) at different coupling strengths ($\lambda$, in a.u.), cavity polarization directions, and basis sets, using a cavity frequency of 0.1 $E_h$ ($\approx$ 2.72 eV).

| Cavity polarization | $\lambda$ | cc-pV*n*Z | | | aug-cc-pV*n*Z | | | d-aug-cc-pV*n*Z | | |
|---|---|---|---|---|---|---|---|---|---|---|
| | | $n = \mathrm{D}$ | $n = \mathrm{T}$ | $n = \mathrm{Q}$ | $n = \mathrm{D}$ | $n = \mathrm{T}$ | $n = \mathrm{Q}$ | $n = \mathrm{D}$ | $n = \mathrm{T}$ | $n = \mathrm{Q}$ |
| None | 0 | −122.340 | −126.262 | −133.060 | −140.371 | −134.834 | −133.899 | −136.009 | −133.465 | −133.117 |
| | 0.01 | −122.607 | −126.555 | −133.378 | −140.768 | −135.236 | −134.303 | −136.426 | −133.870 | −133.522 |
| | 0.02 | −123.400 | −127.426 | −134.321 | −141.944 | −136.424 | −135.496 | −137.660 | −135.067 | −134.715 |
| $x$ | 0.03 | −124.700 | −128.852 | −135.866 | −143.856 | −138.352 | −137.430 | −139.656 | −137.004 | −136.648 |
| | 0.04 | −126.472 | −130.796 | −137.971 | −146.434 | −140.947 | −140.028 | −142.331 | −139.600 | −139.242 |
| | 0.05 | −128.669 | −133.207 | −140.577 | −149.594 | −144.115 | −143.195 | −145.592 | −142.764 | −142.405 |
| | 0.01 | −122.369 | −126.295 | −133.096 | −140.474 | −134.963 | −134.041 | −136.179 | −133.620 | −133.273 |
| | 0.02 | −122.457 | −126.392 | −133.203 | −140.775 | −135.341 | −134.457 | −136.676 | −134.073 | −133.727 |
| $y$ | 0.03 | −122.602 | −126.552 | −133.379 | −141.253 | −135.937 | −135.109 | −137.455 | −134.780 | −134.436 |
| | 0.04 | −122.804 | −126.775 | −133.622 | −141.875 | −136.710 | −135.952 | −138.454 | −135.687 | −135.344 |
| | 0.05 | −123.064 | −127.059 | −133.929 | −142.603 | −137.609 | −136.927 | −139.606 | −136.733 | −136.390 |
| | 0.01 | −121.017 | −124.909 | −131.636 | −138.733 | −133.310 | −132.419 | −134.557 | −132.039 | −131.700 |
| | 0.02 | −117.193 | −120.997 | −127.525 | −134.026 | −128.927 | −128.160 | −130.353 | −127.917 | −127.601 |
| $z$ | 0.03 | −111.262 | −114.937 | −121.166 | −126.807 | −122.199 | −121.609 | −123.829 | −121.525 | −121.242 |
| | 0.04 | −103.778 | −107.301 | −113.171 | −117.827 | −113.817 | −113.425 | −115.605 | −113.477 | −113.228 |
| | 0.05 | −95.972 | −98.705 | −104.193 | −107.859 | −104.491 | −104.290 | −106.356 | −104.433 | −104.218 |
